# Supplementary material for: Improving Your Graph Neural Networks: A High-Frequency Booster
Source: arXiv:2210.08251 source file (2023-05-03)
Supplement: Supplementary file 1 [file 8_appendix.tex]

\clearpage
\newpage
\onecolumn
\appendix
